# Supplementary material for: Discerning quantum memories based on electromagnetically-induced-transparency and Autler-Townes-splitting protocols
Source: arXiv:1902.02815 ancillary file (2019-02-07)
Supplement: Supplementary file 1 [file Captions_for_animations.pdf]

### Description for the animations

The animations show the coherence dynamics associated with on-demand operations of the narrow- and broadband EIT memories, and the broadband ATS memory, under the “backward retrieval” configuration, whereby the stored and subsequently recalled output photonic mode is emitted in the counter-propagating direction to the input photonic mode. The parameters for these animations are identical to those in Figure 2. The left window symbolises free space with the input and output signals, while the right window symbolises the storage medium, with the dynamical evolution of spin  $|S(z, t)|^2$  (blue), polarization  $|P(z, t)|^2$  (orange) and photonic  $|E(z, t)|^2$  (red) coherences. The dashed green curve shows the on/off control field, which initiates the storage and recall processes. Distances in the left and right window panes are not on scale. For each memory implementation, the parameters  $(d, \Omega_C^{pk})$  are optimized to give a 90% memory efficiency.

### Narrowband EIT memory

The input is a narrowband Gaussian pulse with  $B = 0.014\Gamma/2\pi$  ( $\tau = 100/\gamma$ ) and  $d = 100$ ,  $\Omega_C^{pk} = 0.5\Gamma$ . The memory implementation falls into the EIT regime, with the signal bandwidth lying inside the transparency window  $\Delta\omega_{EIT} = 0.025\Gamma$ , such that no signal absorption occurs. This is also apparent from the evolution of coherences, where the reversible mapping between the photonic and spin modes occurs without the excitation of the atomic polarization. The coherence dynamics also show the in-phase relationship between the E and S components. Another important feature of EIT memory is associated with the spatial profile of the spin-wave: the slow-light mediated storage results in a spin-wave that is compressed / localized inside the storage medium, which is in contrast to the ATS memory. Finally, the narrowband EIT implementation is optimal as the adiabaticity condition of  $\tau d\gamma \gg 1$  is fulfilled by having  $\tau d\gamma = 10^4$ .

### Broadband EIT memory

The input is a broadband Gaussian pulse with  $B = 14\Gamma/2\pi$  ( $\tau = 0.1/\gamma$ ) and  $d = 600$ ,  $\Omega_C^{pk} = 55\Gamma$ . Here, the memory implementation falls into the ATS regime, and by choosing  $\Omega_C^{pk}/2\pi = 4B$ , the input signal lies inside the wide transparency between the ATS peaks, such that the absorption is minimised. The time evolution of coherences clearly show that the dynamics of both narrow- and broadband EIT protocols are same. However, the technical resources required to implement an efficient, broadband EIT memory are significantly high. This also follows from the adiabaticity condition, which in this example is fulfilled via  $\tau d\gamma = 60 \gg 1$ .

### Broadband ATS memory

The input is a broadband Gaussian pulse with  $B = 14\Gamma/2\pi$  ( $\tau = 0.1/\gamma$ ) and  $d = 100$ ,  $\Omega_C^{pk} = 14\Gamma$ . The memory implementation is absorption-mediated and thus, requires a significant overlap between the input signal and ATS peaks. This is also visible from the excitation of the polarization coherence during the storage and recall processes. The dynamics also show that at any point inside the medium, when the spin is maximum (minimum), the photonic component is minimum (maximum), i.e. the E and S components are 90 degrees out-of-phase with each other. Further, the spin-wave exhibits an exponentially decaying profile along the medium. Finally, we note that the ATS memory is inherently non-adiabatic in nature for optimal operation, i.e. requires  $\tau d\gamma \sim 1$ . In this example, the condition is fulfilled via  $\tau d\gamma = 10$ .

Comparing with the broadband EIT memory, the ATS memory significantly relaxes the constraints on optical depth and control intensity.
